# Supplementary material for: An efficient and flexible inference system for serving heterogeneous ensembles of deep neural networks
Source: arXiv:2208.14049 source file (2022-08-30)
Supplement: Supplementary file 1 [file appendix_1_algo.tex]

\section{Allocation optimizer algorithl}
\label{sec:algopt}

The goal of the \textit{allocation optimizer} is to found a good solution for the formula~\ref{eq:max}.
\begin{equation}
    A* = \argmax_{A \in \Omega} bench(A,calib\_data) 
    \label{eq:max}
\end{equation}
$\Omega$ is the space of all possible allocation matrices.
