# Supplementary material for: An efficient and flexible inference system for serving heterogeneous ensembles of deep neural networks
Source: arXiv:2208.14049 source file (2022-08-30)
Supplement: Supplementary file 2 [file appendix_2_matrix.tex]

\clearpage
